# Supplementary material for: Topological defects lead to energy transfer in active nematics
Source: arXiv:2411.18214 source file (2025-11-06)
Supplement: Supplementary file 1 [file SI.pdf]

# SI Appendix for Topological defects lead to energy transfer in active nematics

## Contents

|                                               |   |
|-----------------------------------------------|---|
| <b>Derivation of energy dissipation terms</b> | 1 |
| Kinetic energy dissipation                    | 1 |
| Total energy dissipation                      | 3 |
| Elastic energy dissipation                    | 4 |
| <b>Distribution of elastic energy</b>         | 5 |
| <b>Estimating state of experimental data</b>  | 6 |
| <b>Supplementary movie captions</b>           | 9 |

## DERIVATION OF ENERGY DISSIPATION TERMS

### Kinetic energy dissipation

The Navier Stokes equation based on the Beris-Edwards theory of nematodynamics is given by:

$$\rho(\partial_t + v_j \cdot \partial_j)v_i = -\partial_j P \delta_{ij} + \partial_j(\sigma_{ij} + \sigma_{ij}^a) = \partial_j \sigma'_{ij} \quad (\text{S1})$$

Where the total stress,  $\sigma'_{ij} = -P\delta_{ij} + \sigma_{ij}^s + \sigma_{ij}^a$ . The traceless symmetric and anti-symmetric stresses are given by:

$$\sigma_{ij}^s = 2\eta u_{ij} + \lambda S H_{ij} + \alpha Q_{ij} + \sigma_{ij}^E \quad (\text{S2})$$

$$\sigma_{ij}^a = Q_{ik} H_{kj} - H_{ik} Q_{kj} \quad (\text{S3})$$

Where  $Q_{ij}$  is the tensorial director field,  $S$  is the scalar order parameter,  $u_{ij} = (\partial_j v_i + \partial_i v_j)/2$  is the symmetric strain rate tensor,  $P$  is the pressure,  $\eta$  is the shear viscosity,  $\lambda$  is the flow alignment parameter and  $\alpha$  is the activity.

$H_{ij}$  is the molecular field defined by  $\mathbf{H} = -\delta F^{LDG}/\delta \mathbf{Q}$  where  $F^{LDG}$  is the Landau De-Gennes free energy, which results in

$$H_{ij} = K \partial_k^2 Q_{ij} + \frac{K}{\epsilon^2} [1 - S^2] Q_{ij} \quad (\text{S4})$$

with  $K$  the single elastic constant and  $\epsilon$  the defect core radius.

$\sigma_{ij}^E$  is the Ericksen stress which is defined as

$$\sigma_{ij}^E = -\partial_i Q_{kl} \frac{\delta F^{LDG}}{\delta \partial_j Q_{kl}} \quad (\text{S5})$$

The kinetic energy is given by  $F_{KE} = \int \frac{1}{2} \rho v_i^2 d^2 r$ . Thus the rate of change of kinetic energy is given by:

$$\dot{F}_{KE} = \partial_t \int \frac{1}{2} \rho v_i^2 d^2 r \quad (\text{S6})$$

$$= \rho \int v_i \partial_t v_i d^2 r \quad (\text{S7})$$

$$= \int v_i \partial_j \sigma'_{ij} - \rho v_i v_j \partial_j v_i d^2 r \quad (\text{S8})$$

$$= \int v_i \partial_j \sigma'_{ij} + \frac{\rho}{2} \partial_j (v_i v_j v_i) d^2 r \quad (\text{S9})$$

$$= - \int \sigma'_{ij} \partial_j v_i d^2 r \quad (\text{S10})$$

We have used the fact that  $\rho$  is constant for incompressible systems, which has also allowed us to re-write the convective term as a divergence. This can be written as a surface term which we neglect. Finally, we perform an integration by parts, again neglecting the surface terms.

We now write the total stress tensor and strain rate as the sum of symmetric and anti-symmetric parts, i.e.  $\partial_j v_i = u_{ij} - \omega_{ij}$  where  $\omega_{ij} = (\partial_i v_j - \partial_j v_i)/2$ , which allows us to write

$$\dot{F}_{KE} = - \int (-P \delta_{ij} + \sigma_{ij}^s + \sigma_{ij}^a) (u_{ij} - \omega_{ij}) d^2 r \quad (\text{S11})$$

$$= - \int u_{ij} \sigma_{ij}^s - \sigma_{ij}^a \omega_{ij} d^2 r \quad (\text{S12})$$

Where the pressure terms drop by the incompressibility condition. Writing out all the terms in full gives the kinetic energy dissipation rate as:

$$\dot{F}_{KE} = - \int 2\eta u_{ij} u_{ij} + \lambda S H_{ij} u_{ij} + \alpha Q_{ij} u_{ij} + \sigma_{ij}^E u_{ij} - \omega_{ij} (Q_{ik} H_{kj} - H_{ik} Q_{kj}) d^2 r \quad (\text{S13})$$

Where we identify the dissipation due to viscosity, flow alignment, active injection, relaxation of

the Ericksen stress, and elastic interaction with the director field respectively as:

$$D_v = -2\eta \int u_{ij} u_{ij} d^2r \quad (\text{S14})$$

$$D_f = -\lambda \int S H_{ij} u_{ij} d^2r \quad (\text{S15})$$

$$I = -\alpha \int Q_{ij} u_{ij} d^2r \quad (\text{S16})$$

$$T_{el} = - \int \sigma_{ij}^E u_{ij} d^2r \quad (\text{S17})$$

$$D_{el} = \int \omega_{ij} (Q_{ik} H_{kj} - H_{ik} Q_{kj}) d^2r \quad (\text{S18})$$

These contributions are plotted in Fourier space in Fig. S1 and we observe no kinetic energy transfer between length scales, as expected at low Reynolds number [? ? ? ].

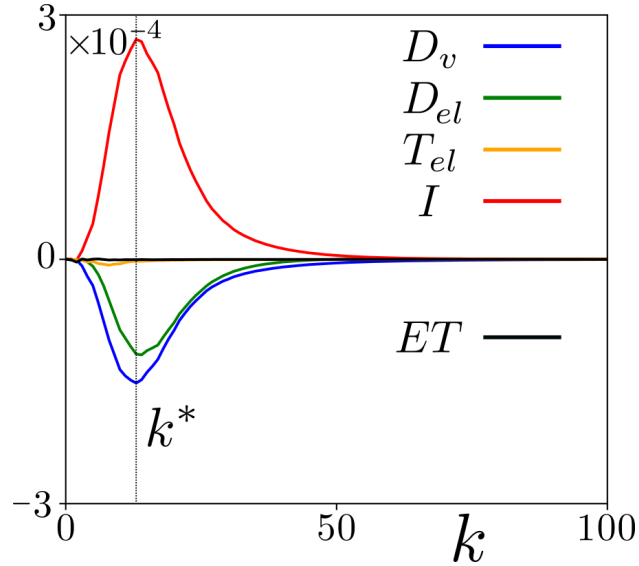

FIG. S1: Dissipation spectra for the kinetic energy of a simulated active nematic based on identical data to that presented in Fig.1 (main text). Since flow alignment is set to zero,  $\lambda = 0$ , we have omitted the corresponding contribution from this figure. The black line shows the kinetic energy transfer between length scales, which remains negligible.

### Total energy dissipation

To obtain the total energy dissipation rate,  $\dot{F} = \dot{F}_{KE} + \dot{F}_{LDG}$  one must follow the framework of linear, non-equilibrium thermodynamics [? ? ]. We follow in more detail here the last few steps to show the source of the change in the energy dissipation. In the case of an isothermal, two dimensional, incompressible fluid in which the Landau De-Gennes free energy describes the director

field, the rate of change of free energy is given by:

$$\dot{F} = - \int \sigma_{ij}^s u_{ij} - \sigma_{ij}^a \omega_{ij} + D_t Q_{ij} H_{ij} \, d^2 r \quad (\text{S19})$$

Substituting in for the material derivative of  $Q$  we derive the additional terms in the dissipation as:

$$\int D_t Q_{ij} H_{ij} d^2 r = \int -\lambda S u_{ij} H_{ij} + \frac{1}{\gamma} H_{ij} H_{ij} + Q_{ik} \omega_{kj} H_{ij} - \omega_{ik} Q_{kj} H_{ij} \, d^2 r \quad (\text{S20})$$

We first see that the first term exactly cancels with  $D_f$  from the kinetic energy dissipation. This is a result of Onsager reciprocity, as the flow alignment is a conservative interaction between the strain rate and the director field. Next we see that, by a relabelling of the indexes, the last two terms exactly cancel with  $D_{el}$ , which is a result of conservation of angular momentum. Thus when we write the total dissipation terms we are left with:

$$D_v = -2\eta \int u_{ij} u_{ij} \, d^2 r \quad (\text{S21})$$

$$D_Q = -\frac{1}{\gamma} \int H_{ij} H_{ij} \, d^2 r \quad (\text{S22})$$

$$I = -\alpha \int Q_{ij} u_{ij} \, d^2 r \quad (\text{S23})$$

$$T_{el} = - \int \sigma_{ij}^E u_{ij} \, d^2 r \quad (\text{S24})$$

### Elastic energy dissipation

As we have shown above, the dissipation of elastic energy is given by:

$$D_Q = -\frac{1}{\gamma} \int H_{ij} H_{ij} \, d^2 r \quad (\text{S25})$$

Where the traceless, symmetric molecular tensor is given by

$$H_{ij} = K \partial_k^2 Q_{ij} + \frac{K}{\epsilon^2} [1 - S^2] Q_{ij} \quad (\text{S26})$$

Substituting this into the elastic dissipation we arrive at

$$D_Q = -\frac{K^2}{\gamma} \int [\partial_k^2 Q_{ij}] [\partial_l^2 Q_{ij}] + \frac{2}{\epsilon^2} [1 - S^2] Q_{ij} \partial_k^2 Q_{ij} + \frac{1}{2\epsilon^4} [S - S^3]^2 \, d^2 r \quad (\text{S27})$$

where we have used the fact that  $[Q_{xx}^2 + Q_{yy}^2] = S^2/4$  in the last term.

We now identify the terms with the different parts of the free energy, i.e.

$$D_Q = D_Q^F + D_Q^{FL} + D_Q^L \quad (\text{S28})$$

The first term is the dissipation of elastic energy stored as distortion of the tensorial director field (identified as  $F^F$  in the main text).

$$D_Q^F = -\frac{K^2}{\gamma} \int [\partial_k^2 Q_{ij}] [\partial_l^2 Q_{ij}] d^2r \quad (\text{S29})$$

$$= -\frac{2K^2}{\gamma} \int [(\partial_x^2 + \partial_y^2) Q_{xx}]^2 + [(\partial_x^2 + \partial_y^2) Q_{xy}]^2 d^2r \quad (\text{S30})$$

Where we have written it as a function of the independent components of the  $Q$  tensor, which we obtain from simulation.

The third term is associated with dissipation of elastic energy stored as deviations of the scalar order parameter (identified as  $F^L$  in the main text).

$$D_Q^L = -\frac{K^2}{2\gamma\epsilon^4} \int [S - S^3]^2 d^2r \quad (\text{S31})$$

where  $S^2 = 4[Q_{xx}^2 + Q_{xy}^2]$ , which we obtain from simulation.

The second term comes from a combination of  $F^F$  and  $F^L$ . This offsets  $D_Q^F$  and  $D_Q^L$  when energy is exchanged between the two.

$$D_Q^{FL} = -\frac{2K^2}{\gamma\epsilon^2} \int [1 - S^2] Q_{ij} \partial_k^2 Q_{ij} d^2r \quad (\text{S32})$$

$$= -\frac{4K^2}{\gamma\epsilon^2} \int [1 - S^2] [Q_{xx}(\partial_x^2 + \partial_y^2) Q_{xx} + Q_{xy}(\partial_x^2 + \partial_y^2) Q_{xy}] d^2r \quad (\text{S33})$$

where once again,  $Q_{xx}$ ,  $Q_{xy}$  and  $S$  are obtained through simulation.

## DISTRIBUTION OF ELASTIC ENERGY

The distribution of stored elastic energy in an active nematic in the defect chaos regime is peaked around the active length scale, but the distribution is exponential as shown in Fig. 1 (main text). We show here that the length scale of this exponential is related to the defect core radius,  $\epsilon$ . Fig. S2a&b show the distribution of energy associated with the distortion (blue) and scalar order parameter (red) for a range of values of  $\epsilon$  that all display an exponential distribution. Upon re-scaling by the defect core radius, we see that the lines become close to parallel, see Fig. S2c&d. We can additionally show this by fitting the tail of the distribution to an exponential of the form  $f(k) \sim \exp(-k/k_0)$ . Plotting  $k_0$  against  $\epsilon$  shows a roughly linear relationship.

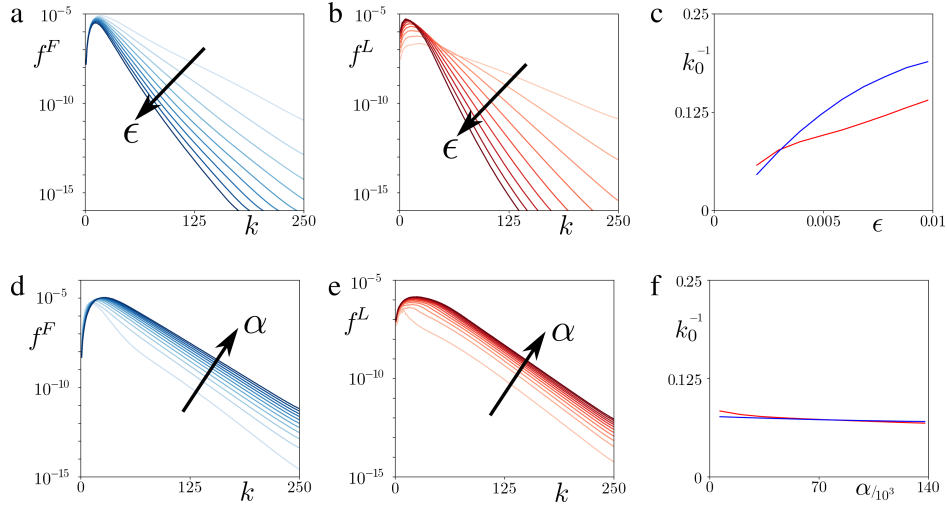

FIG. S2: (a&b) Elastic energy spectra during defect chaos showing the distortion ( $f_F$ ) and scalar order parameter ( $f_L$ ) contributions to the Landau De-Gennes free energy for  $\epsilon$  varying from  $1/512$  to  $5/512$  ( $\alpha = 0.125 \times 512^2$ ). (c) by fitting the tails of the distributions in (a&b) to an exponential distribution  $f \sim \exp[-k/k_0]$  we can extract a characteristic length scale  $k_0^{-1}$  which appears to scale with the defect core radius ( $\epsilon$ ). (d&e) same as (a&b) for varying  $\alpha$  from  $0.025 \times 512^2$  to  $0.525 \times 512^2$  ( $\epsilon = 1.5/512$ ). (f) Using the same process as (c) we extract a characteristic length scale,  $k_0^{-1}$ , from the energy distribution which does not appear to vary greatly with activity.

### ESTIMATING STATE OF EXPERIMENTAL DATA

We use data in which a two dimensional, microtubule-based active nematic is studied experimentally (see Movie S3). In the experiments, the local orientation of filaments is estimated by measuring, in real time, the local birefringence or the active layer [? ]. This can also be used to provide a measure of the local order parameter,  $S$ . In the following section we show how this data can be used to place the experiments within the context of our numerical results.

We introduce  $q_{\alpha\beta} = Q_{\alpha\beta}/S$  with  $q_{\alpha\beta}^2 = 1/2$ . We now re-write the Landau De-Gennes free energy in these terms giving:

$$F = \int \frac{K}{2} [\partial_k S q_{ij}]^2 + \frac{K}{4\epsilon^2} S^2 - \frac{K}{8\epsilon^2} S^4 \, d^2 r \quad (\text{S34})$$

$$= \int \frac{K}{2} [q_{ij} \partial_k S + S \partial_k q_{ij}]^2 + \frac{K}{4\epsilon^2} S^2 - \frac{K}{8\epsilon^2} S^4 \, d^2 r \quad (\text{S35})$$

$$= \int \frac{K}{2} [q_{ij}^2 (\partial_k S)^2 + S^2 (\partial_k q_{ij})^2 + 2S \partial_k S q_{ij} \partial_k q_{ij}] + \frac{K}{4\epsilon^2} S^2 - \frac{K}{8\epsilon^2} S^4 \, d^2 r \quad (\text{S36})$$

$$(\text{S37})$$

In the interest of compactness, we define the following fields

$$G_k = q_{ij} \partial_k q_{ij} \quad (\text{S38})$$

$$J = (\partial_k q_{ij})^2 \quad (\text{S39})$$

Which allows us to write

$$F = \int \frac{K}{2} \left[ \frac{1}{2} (\partial_k S)^2 + S^2 J + 2SG_k \partial_k S \right] + \frac{K}{4\epsilon^2} S^2 - \frac{K}{8\epsilon^2} S^4 \, d^2 r \quad (\text{S40})$$

We can now minimize the free energy with respect to the order parameter with simple relaxation dynamics given by:

$$\partial_t S = \frac{\delta F}{\delta S} \quad (\text{S41})$$

Where  $\frac{\delta F}{\delta S}$  is the functional derivative of the Landau De-Gennes free energy with respect to the order parameter, given by:

$$\frac{\delta F}{\delta S} = KS[J - \partial_k G_k] - \frac{K}{2} \partial_k^2 S + \frac{K}{2\epsilon^2} S[1 - S^2] \quad (\text{S42})$$

Thus for a given orientational field  $\theta$ , we can calculate the  $S(\epsilon)$  field that minimizes the Landau De-Gennes free energy for a specific value of  $\epsilon$ . Note here, because  $\frac{\delta F}{\delta S}$  is linear in  $K$  it does not affect the outcome of this process.

We use the above equation to generate an estimated order parameter for orientation fields measured in an experimentally realized microtubule-based active nematic for a specific value of  $\epsilon$ , which we denote  $S(\epsilon)$ . We can calculate the error in the estimation of  $S(\epsilon)$  by comparing it with the order parameter measured in experiments,  $S^{\text{exp}}$ , given by:

$$E(\epsilon) = \int (S(\epsilon) - S^{\text{exp}})^2 d^2 r \quad (\text{S43})$$

We estimate  $\epsilon$  as the value that minimizes  $E(\epsilon)$ , which we calculate as  $\epsilon = 1.2\text{pixels}$ .

We calculate the winding number at each pixel to measure the average number of topological defects visible within the frame, which comes to  $\langle N \rangle = 119.5$ . We construct a characteristic separation length between defects as  $l = \sqrt{A/\langle N \rangle}$ . The area of the image is  $102 \times 127\text{pixels}$ , which gives an inter defect length scale of  $l = 10.4\text{pixels}$ . We combine this to give a dimensionless inter defect spacing of  $l/\epsilon = 8.66$ .

We can perform an identical analysis of our simulation results since the simulation area  $A$  is exactly known and the number of defects can be counted again by calculating the winding number. When this is compared with  $\epsilon$  for the same simulations we identify a line through parameter space on which the inter defect distance and the defect core radius are the same as that observed in experiments, this is shown as a pink line in Fig. 3 (main text).

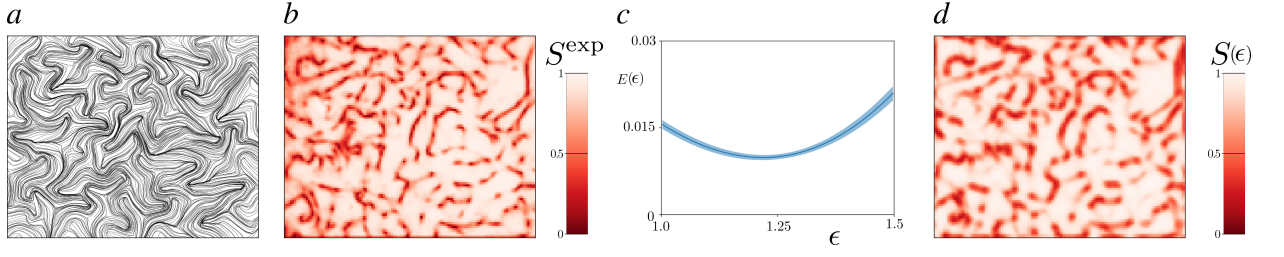

FIG. S3: (a) Orientation field and (b) Scalar order parameter taken from a typical kinesin/microtubule-based active nematic experiment. (c) Error in the Scalar order parameter that minimizes the Landau De-Gennes energy for a director field taken from experiments for different values of  $\epsilon$ . (d) Scalar order parameter that minimizes the Landau De-Gennes free energy for the director field given in (a);  $\epsilon = 1.2$ .

# SUPPLEMENTARY MOVIE CAPTIONS

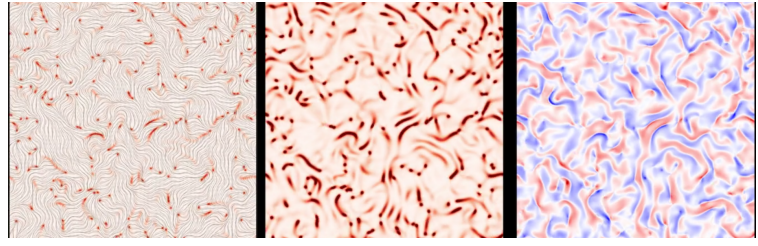

Movie S1: Simulated active nematic corresponding to the data shown in Fig. 1 of the main text. Panels correspond to the director field lines overlaid to the scalar order parameter (left), scalar order parameter with enhanced contrast (center), and vorticity field (right).

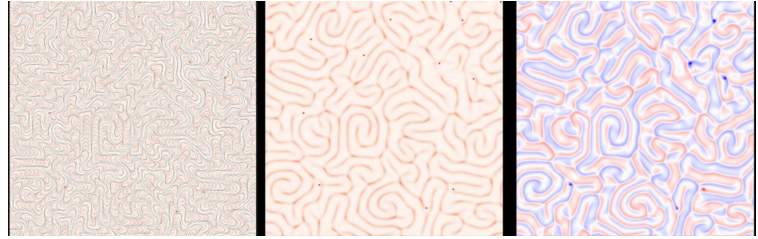

Movie S2: Simulated active nematic corresponding to the data shown in Fig. 4 of the main text. Panels correspond to the director field lines overlaid to the scalar order parameter (left), scalar order parameter with enhanced contrast (center), and vorticity field (right).

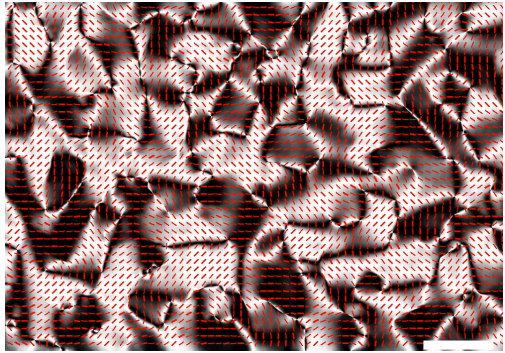

Movie S3: Rendering of the orientational field extracted from an experiment with a kinesin/microtubule active nematic. See Ref. [? ]. The coarse-grained director field is overlaid on the corresponding schlieren texture. The scalebar is  $200\ \mu\text{m}$ .
